# Supplementary material for: VideoNSA: Native Sparse Attention Scales Video Understanding
Source: arXiv:2510.02295 source file (2026-01-30)
Supplement: Supplementary file 1 [file slc_complex.tex]

\section{Complexity of the Selection Branch.}
Let the sequence length be $L$, and assume keys/values are partitioned into blocks of size $b$. 
For each query, the selection branch identifies the top-$N$ blocks (corresponding to $S = N \cdot b$ tokens) using importance scores computed from the compression branch.

\textbf{(1) Importance scoring and top-$k$ reduction.} 
Each query must evaluate scores over all $L/b$ blocks and perform an online top-$k$ reduction. 
With $L$ queries in total, the arithmetic and memory complexity becomes
\[
T_{\text{score+topk}} = \Theta\!\left(L \cdot \frac{L}{b}\right) = \Theta\!\left(\tfrac{L^2}{b}\right).
\]
This quadratic-like term is the dominant source of inefficiency as $L$ grows. 
The additional $\log N$ factor for heap maintenance is negligible in practice since $N$ is fixed.

\textbf{(2) Attention over the selected subset.} 
Once the top-$N$ blocks are identified, each query attends only to its selected subset. 
The cost of scaled dot-product attention is therefore
\[
T_{\text{attn(selected)}} = \Theta(L \cdot S) = \Theta(L \cdot N b),
\]
which scales linearly with $L$ when $S$ is constant.

\textbf{(3) Backward computation.} 
We adopt a two-pass design that reconstructs the reverse mapping from keys/values to queries. 
This effectively doubles the linear $O(L \cdot S)$ work of the forward pass and introduces additional memory access, 
but it does not change the $O(L^2/b)$ complexity from the scoring stage.

\textbf{Overall.} 
The total complexity of the selection branch can thus be summarized as
\[
T_{\text{select}}(L) = \underbrace{\Theta(L^2/b)}_{\text{scoring and top-}k} \;+\; 
\underbrace{\Theta(L \cdot S)}_{\text{selected attention (fwd/bwd)}}.
\]
Although the attention on the reduced subset is near-linear, the per-query sweep over all blocks makes the selection branch approach quadratic scaling in practice. 
This effect is further exacerbated by non-coalesced memory accesses, atomic operation overheads, and the additional passes required in the backward kernel. 
Consequently, the selection branch becomes the primary efficiency bottleneck under long-context settings.
